# Supplementary material for: 3R-GS: Best Practice in Optimizing Camera Poses Along with 3DGS
Source: arXiv:2504.04294 source file (2025-04-05)
Supplement: Supplementary file 1 [file supp-pose.tex]

\begin{table*}[h]
    \centering
    \vspace{-0.3cm}
    \resizebox{\textwidth}{!}{ % Ensures the table fits within two columns
\begin{tabular}{
>{\columncolor[HTML]{FFFFFF}}c 
>{\columncolor[HTML]{FFFFFF}}c 
>{\columncolor[HTML]{FFFFFF}}c 
>{\columncolor[HTML]{FFFFFF}}c 
>{\columncolor[HTML]{FFFC9E}}c 
>{\columncolor[HTML]{FFFC9E}}c 
>{\columncolor[HTML]{FFFFFF}}c 
>{\columncolor[HTML]{FFCE93}}c 
>{\columncolor[HTML]{FFCE93}}c 
>{\columncolor[HTML]{FFFFFF}}c 
>{\columncolor[HTML]{FFCCC9}}c 
>{\columncolor[HTML]{FFCCC9}}c 
>{\columncolor[HTML]{FFFFFF}}c }
\hline
\cellcolor[HTML]{FFFFFF}                         & \multicolumn{2}{c}{\cellcolor[HTML]{FFFFFF}3DGS}             &  & \multicolumn{2}{c}{\cellcolor[HTML]{FFFFFF}3DGS-MCMC}                 &  & \multicolumn{2}{c}{\cellcolor[HTML]{FFFFFF}3DGS-MCMC + $\mathcal{R}_{\text{MLP}}$}                 &  & \multicolumn{2}{c}{\cellcolor[HTML]{FFFFFF}3DGS-MCMC + $\mathcal{R}_{\text{MLP}}$  + $\mathcal{L}_{\text {geo}}$}                 &  \\ \cline{2-3} \cline{5-6} \cline{8-9} \cline{11-12}
\multirow{-2}{*}{\cellcolor[HTML]{FFFFFF}Scenes} & Rotation(°)                  & ATE (m)                       &  & \cellcolor[HTML]{FFFFFF}Rotation(°) & \cellcolor[HTML]{FFFFFF}ATE (m) &  & \cellcolor[HTML]{FFFFFF}Rotation(°) & \cellcolor[HTML]{FFFFFF}ATE (m) &  & \cellcolor[HTML]{FFFFFF}Rotation(°) & \cellcolor[HTML]{FFFFFF}ATE (m) &  \\ \hline
Truck                                            & 0.83                         & 0.027                         &  & 0.81                                & 0.025                           &  & 0.27                                & 0.017                           &  & 0.16                                & 0.011                           &  \\
Ignatius                                         & 0.23                         & 0.016                         &  & 0.20                                & 0.014                           &  & 0.11                                & 0.008                           &  & 0.06                                & 0.005                           &  \\
Cartpillar                                       & 1.41                         & 0.402                         &  & 1.40                                & 0.040                           &  & 0.62                                & 0.034                           &  & 0.32                                & 0.020                           &  \\
Meetingroom                                      & 0.75                         & 0.052                         &  & 0.72                                & 0.048                           &  & 0.41                                & 0.040                           &  & 0.24                                & 0.023                           &  \\ \hline
garden                                           & \cellcolor[HTML]{FFFC9E}0.19 & \cellcolor[HTML]{FFCE93}0.003 &  & \cellcolor[HTML]{FFCE93}0.16        & \cellcolor[HTML]{FFCCC9}0.002   &  & \cellcolor[HTML]{FFCCC9}0.03        & \cellcolor[HTML]{FFCCC9}0.002   &  & 0.03                                & 0.002                           &  \\
counter                                          & 0.25                         & \cellcolor[HTML]{FFFC9E}0.011 &  & 0.23                                & 0.011                           &  & 0.11                                & 0.008                           &  & 0.05                                & 0.003                           &  \\
bicycle                                          & 1.07                         & 0.034                         &  & 1.03                                & 0.029                           &  & 0.59                                & 0.018                           &  & 0.09                                & 0.013                           &  \\
room                                             & 0.27                         & \cellcolor[HTML]{FFCE93}0.016 &  & 0.26                                & \cellcolor[HTML]{FFCE93}0.016   &  & 0.16                                & 0.016                           &  & 0.13                                & 0.012                           &  \\ \hline
scan69                                           & 0.23                         & \cellcolor[HTML]{FFFC9E}0.006 &  & 0.23                                & 0.006                           &  & 0.18                                & 0.004                           &  & 0.10                                & 0.003                           &  \\
scan106                                          & \cellcolor[HTML]{FFCE93}0.13 & \cellcolor[HTML]{FFCE93}0.004 &  & \cellcolor[HTML]{FFCE93}0.13        & \cellcolor[HTML]{FFCE93}0.004   &  & 0.13                                & \cellcolor[HTML]{FFCCC9}0.003   &  & 0.11                                & 0.003                           &  \\
scan110                                          & 0.48                         & 0.007                         &  & 0.47                                & 0.007                           &  & 0.17                                & 0.005                           &  & 0.13                                & 0.004                           &  \\
scan83                                           & 0.26                         & 0.007                         &  & 0.27                                & 0.008                           &  & 0.21                                & 0.007                           &  & 0.19                                & 0.005                           &  \\ \hline
\end{tabular}    }
    %\vspace{-1pt}
    \vspace{-0.3cm}
\caption{Per-scene ablation study results for novel view synthesis.}
    \label{tab: supp-pose}
\end{table*}
