# Supplementary material for: 3R-GS: Best Practice in Optimizing Camera Poses Along with 3DGS
Source: arXiv:2504.04294 source file (2025-04-05)
Supplement: Supplementary file 2 [file supp-visual.tex]

\begin{table*}[h]
    \centering
    \vspace{-0.3cm}
    \resizebox{\textwidth}{!}{ % Ensures the table fits within two columns
\begin{tabular}{
>{\columncolor[HTML]{FFFFFF}}c 
>{\columncolor[HTML]{FFFFFF}}c 
>{\columncolor[HTML]{FFFFFF}}c 
>{\columncolor[HTML]{FFFFFF}}c 
>{\columncolor[HTML]{FFFFFF}}l 
>{\columncolor[HTML]{FFFC9E}}c 
>{\columncolor[HTML]{FFFC9E}}c 
>{\columncolor[HTML]{FFFC9E}}c 
>{\columncolor[HTML]{FFFFFF}}l 
>{\columncolor[HTML]{FFCE93}}c 
>{\columncolor[HTML]{FFCE93}}c c
>{\columncolor[HTML]{FFFFFF}}l 
>{\columncolor[HTML]{FFCCC9}}c 
>{\columncolor[HTML]{FFCCC9}}c 
>{\columncolor[HTML]{FFCCC9}}c }
\hline
\cellcolor[HTML]{FFFFFF}                         & \multicolumn{3}{c}{\cellcolor[HTML]{FFFFFF}3DGS}                      &  & \multicolumn{3}{c}{\cellcolor[HTML]{FFFFFF}3DGS-MCMC}                                         &  & \multicolumn{3}{c}{\cellcolor[HTML]{FFFFFF}3DGS-MCMC + $\mathcal{R}_{\text{MLP}}$ }                                     &  & \multicolumn{3}{c}{\cellcolor[HTML]{FFFFFF}3DGS-MCMC + $\mathcal{R}_{\text{MLP}}$  + $\mathcal{L}_{\text {geo}}$}                                 \\ \cline{2-4} \cline{6-8} \cline{10-12} \cline{14-16} 
\multirow{-2}{*}{\cellcolor[HTML]{FFFFFF}Scenes} & PSNR  & SSIM                          & LPIPS                         &  & \cellcolor[HTML]{FFFFFF}PSNR  & \cellcolor[HTML]{FFFFFF}SSIM  & \cellcolor[HTML]{FFFFFF}LPIPS &  & \cellcolor[HTML]{FFFFFF}PSNR  & \cellcolor[HTML]{FFFFFF}SSIM  & \cellcolor[HTML]{FFFFFF}LPIPS &  & \cellcolor[HTML]{FFFFFF}PSNR  & \cellcolor[HTML]{FFFFFF}SSIM  & \cellcolor[HTML]{FFFFFF}LPIPS \\ \hline
Truck                                            & 20.91 & 0.723                         & 0.181                         &  & 22.40                         & 0.770                         & 0.158                         &  & 24.37                         & 0.843                         & \cellcolor[HTML]{FFCE93}0.129 &  & 24.82                         & 0.860                         & 0.121                         \\
Ignatius                                         & 18.96 & 0.665                         & 0.249                         &  & 21.69                         & 0.758                         & 0.210                         &  & \cellcolor[HTML]{FFCCC9}21.98 & 0.767                         & \cellcolor[HTML]{FFCE93}0.201 &  & \cellcolor[HTML]{FFCE93}21.93 & 0.778                         & 0.198                         \\
Cartpillar                                       & 19.29 & 0.539                         & 0.349                         &  & 19.89                         & 0.562                         & 0.291                         &  & 22.79                         & 0.736                         & \cellcolor[HTML]{FFCE93}0.250 &  & 23.37                         & 0.773                         & 0.235                         \\
Meetingroom                                      & 22.78 & 0.784                         & 0.239                         &  & 23.79                         & 0.804                         & 0.230                         &  & 25.28                         & 0.865                         & \cellcolor[HTML]{FFCE93}0.191 &  & 25.93                         & 0.867                         & 0.177                         \\ \hline
garden                                           & 24.85 & 0.729                         & 0.126                         &  & 24.53                         & 0.713                         & 0.157                         &  & 25.87                         & 0.804                         & \cellcolor[HTML]{FFCE93}0.150 &  & 26.44                         & 0.820                         & 0.131                         \\
counter                                          & 27.57 & 0.862                         & 0.209                         &  & \cellcolor[HTML]{FFCE93}28.63 & \cellcolor[HTML]{FFCE93}0.891 & \cellcolor[HTML]{FFCE93}0.166 &  & \cellcolor[HTML]{FFFC9E}28.35 & \cellcolor[HTML]{FFFFC7}0.883 & \cellcolor[HTML]{FFFC9E}0.169 &  & 28.80                         & 0.897                         & 0.157                         \\
bicycle                                          & 17.52 & 0.303                         & 0.567                         &  & 17.50                         & 0.294                         & 0.454                         &  & 20.82                         & 0.452                         & \cellcolor[HTML]{FFCE93}0.378 &  & 24.89                         & 0.727                         & 0.252                         \\
room                                             & 30.66 & \cellcolor[HTML]{FFFC9E}0.899 & \cellcolor[HTML]{FFFC9E}0.204 &  & 31.75                         & \cellcolor[HTML]{FFCE93}0.921 & \cellcolor[HTML]{FFCE93}0.158 &  & 31.73                         & 0.921                         & \cellcolor[HTML]{FFCCC9}0.154 &  & 31.82                         & 0.924                         & 0.154                         \\ \hline
scan69                                           & 26.37 & 0.865                         & \cellcolor[HTML]{FFFC9E}0.134 &  & 26.43                         & 0.860                         & \cellcolor[HTML]{FFCE93}0.112 &  & 26.49                         & \cellcolor[HTML]{FFCCC9}0.871 & \cellcolor[HTML]{FFCCC9}0.109 &  & 26.62                         & \cellcolor[HTML]{FFCE93}0.868 & \cellcolor[HTML]{FFCE93}0.112 \\
scan106                                          & 32.74 & 0.923                         & \cellcolor[HTML]{FFFC9E}0.109 &  & 34.15                         & 0.933                         & \cellcolor[HTML]{FFCE93}0.066 &  & \cellcolor[HTML]{FFCCC9}34.67 & 0.935                         & \cellcolor[HTML]{FFCCC9}0.064 &  & \cellcolor[HTML]{FFCE93}34.35 & 0.936                         & \cellcolor[HTML]{FFCE93}0.066 \\
scan110                                          & 31.46 & 0.905                         & 0.142                         &  & 31.55                         & 0.918                         & 0.087                         &  & 32.46                         & 0.928                         & \cellcolor[HTML]{FFCCC9}0.072 &  & 32.63                         & 0.931                         & \cellcolor[HTML]{FFCE93}0.074 \\
scan83                                           & 28.36 & 0.882                         & 0.172                         &  & 27.89                         & \cellcolor[HTML]{FFCE93}0.875 & 0.121                         &  & \cellcolor[HTML]{FFCCC9}28.66 & \cellcolor[HTML]{FFFC9E}0.871 & \cellcolor[HTML]{FFCCC9}0.115 &  & \cellcolor[HTML]{FFCE93}28.44 & 0.881                         & \cellcolor[HTML]{FFCE93}0.117 \\ \hline
\end{tabular}
    }
    %\vspace{-1pt}
    \vspace{-0.3cm}
\caption{Per-scene ablation study results for camera pose registration.}
    \label{tab: supp-visual}
\end{table*}
